# Supplementary material for: Social Context-aware GCN for Video Character Search via Scene-prior Enhancement
Source: arXiv:2305.12348 source file (2023-05-21)
Supplement: Supplementary file 1 [file appendix.tex]

\section{Appendix}
\subsection{Datasets and Pre-processing}
We construct two datasets for characters search task based on movies collected from Bilibili-Relation\cite{zhou2019character} and MovieNet dataset\cite{huang2020movienet}.\par

\textbf{Social-Bilibili Dataset}. The dataset contains 70 films with an average length of 2 hours, 375 main characters, related subtitles and screen-bullet comments. According to \cite{zhou2019character}, all relationships are grouped into five categories, which are working, kinship, hostile, friend and couple respectively. Besides, they label all the characters' relationships and corresponding appearance time. Based on the dataset, we sampled 325 characters, a total of 11478 images, for train, and the remaining 50 characters, 1989 images, for test. Following \cite{li2021social}, we selected a clear image for each character as the query image, which constitutes our query set. In addition, we collect the video frames and textual information with time window $T_t=[t-12, t+12]$ as the context. Moreover, because social context-aware methods need relationships between gallery characters, those scenes in the test set with less than two characters will be filtered out. The dataset is specifically described as Table \ref{bldataset}.\par
\begin{table}
	\begin{center}
		\caption{Social-Bilibili Dataset}
		\label{bldataset}
		\begin{tabular}{l|ccc}
			\toprule
			& Train & Test & Query \\
			\midrule
			Num of images & 11,461 & 1,989 & 375 \\
			Num of identities & 325 & 50 & 375\\
			Num of frames & 183,376 & 31,824 & 6,016\\
			Num of subtitles & 53,637 & 9,368 & 1,510\\
			Num of comments & 184,866 & 32,003 & 6,080\\
			\bottomrule
		\end{tabular}
	\end{center}
\end{table}

\begin{table}
	\begin{center}
		\caption{Social-MovieNet Dataset}
		\label{mvdataset}
		\begin{tabular}{l|ccc}
			\toprule
			& Train & Test & Query \\
			\midrule
			Num of images & 14,462 & 5991 & 79 \\
			Num of identities & 59 & 20 & 79 \\
			Num of frames & 144,606 & 59,904 & 790 \\
			Num of subtitles & 49,191 & 21,358 & 282\\
			Num of comments & - & - & -\\
			\bottomrule
		\end{tabular}
	\end{center}
\end{table}
\textbf{Social-MovieNet Dataset}. We collected social relation graphs for 16 films from MovieNet, with an average length of 1.7 hours, 79 main characters and related subtitles. To be consistent with the Social-BiliBili dataset, we also group all relationships into five categories, which are working, kinship, hostile, friend and couple respectively. We sampled 59 characters, a total of 14462 images, for train, and the remaining 20 characters, 5991 images, for test. Similarly, we selected a clear image for each character as a query image, which constitutes our query set. Since MovieNet has split movies into shots, we set the time window to $T_t=[t-2, t+2]$, where $t$ is the id of the shot. All frames and subtitles in $T_t$ will be collected as the context. The dataset is specifically described as Table \ref{mvdataset}.

\subsection{Ablation Study on Social-MovieNet Dataset}
\begin{table}
	\begin{center}
		\caption{The Performance of Our Method with Different Visual Backbones on Social-MovieNet Dataset}
		\label{ablationvbb2}
		\begin{tabular}{c|c|c|c|c}
			\toprule
			Method & Backbone & mAP & mINP & R1 \\
			\midrule
			\midrule
			ResNet & ResNet50 & 42.0 & 22.2 & 65.0 \\
			ResNet-mid & ResNet50 & 45.0 & 22.0 & 75.0 \\
			TransReID & DeiT-S/16 & 46.7 & 21.7 & 85.0 \\
			TransReID & DeiT-B/16 & 53.5 & 22.3 & 90.0 \\
			TransReID & ViT-S/16 & 46.9 & 22.1 & 80.0 \\
			TransReID & ViT-B/16 & 62.3 & \textbf{24.6} & 90.0 \\
			\midrule
			\midrule
			SoCoSearch & ResNet50 & 41.5 & 22.1 & 70.0 \\
			SoCoSearch & ResNet-mid & 43.2 & 21.9 & 70.0 \\
			SoCoSearch & DeiT-S/16 & 48.7 & 22.0 & 90.0 \\
			SoCoSearch & DeiT-B/16 & 55.1 & 22.8 & 90.0 \\
			SoCoSearch & ViT-S/16 & 46.5 & 22.3 & 75.0 \\
			SoCoSearch & ViT-B/16 & \textbf{63.6} & 24.5 & \textbf{95.0} \\
			\bottomrule
		\end{tabular}
	\end{center}
\end{table}
On the Social-MovieNet dataset, although most backbones have improved after being equipped with social context-aware GCN, the performance of ResNet and ResNet-mid decreased. As mentioned earlier, we select anchor nodes through identity probability, and the selection of anchor nodes will affect the performance of the model. In addition, mAP can reflect the average level of whether the identity probability of each gallery is accurate. However, the two models are all too low on mAP, which affects the selection of anchor nodes and ultimately leads to the decline of model performance.\par

We also compare the performance of our model with different modal information on Social-MovieNet dataset.For models that do not use both visual and textual contexts, it can be regarded as the TransReID, which only depends on the image features to match characters. It can be seen that when the task is difficult, the anchor selection become less accurate, thus, adding social information reduces the mINP to some extent. Fortunately, The dynamic adjustment of feature weight makes mINP decrease by only 0.1\, while mAP and R1 increase by 1.5\% and 5.0\% respectively. In addition, according to mAP and R1, when just using visual or textual information, the model is still effective, but the performance will be slightly decreased compared with the model with both modalities. It is necessary to integrate the multimodal clues for better performance. 
\par
\begin{table}
	\begin{center}
		\caption{The Performance of Our Method with Different Modal Information on Social-MovieNet Dataset}
		\label{ablationrbb2}
		\begin{tabular}{c|c|c|c|c|c}
			\toprule
			Method & Visual & Textual & mAP & mINP & R1 \\
			\midrule
			\midrule
			w/o VT & - & - & 62.3 & \textbf{24.6} & 90.0 \\
			w/o V & - & Bert & 63.7 & 24.5 & 95.0 \\
			w/o T & TSM & - & 63.7 & 24.3 & 95.0 \\
			all & TSM & Bert & \textbf{63.8} & 24.5 & \textbf{95.0} \\
			\bottomrule
		\end{tabular}
	\end{center}
\end{table}

\begin{figure}[h]
	\centering
	\includegraphics[width=\linewidth]{./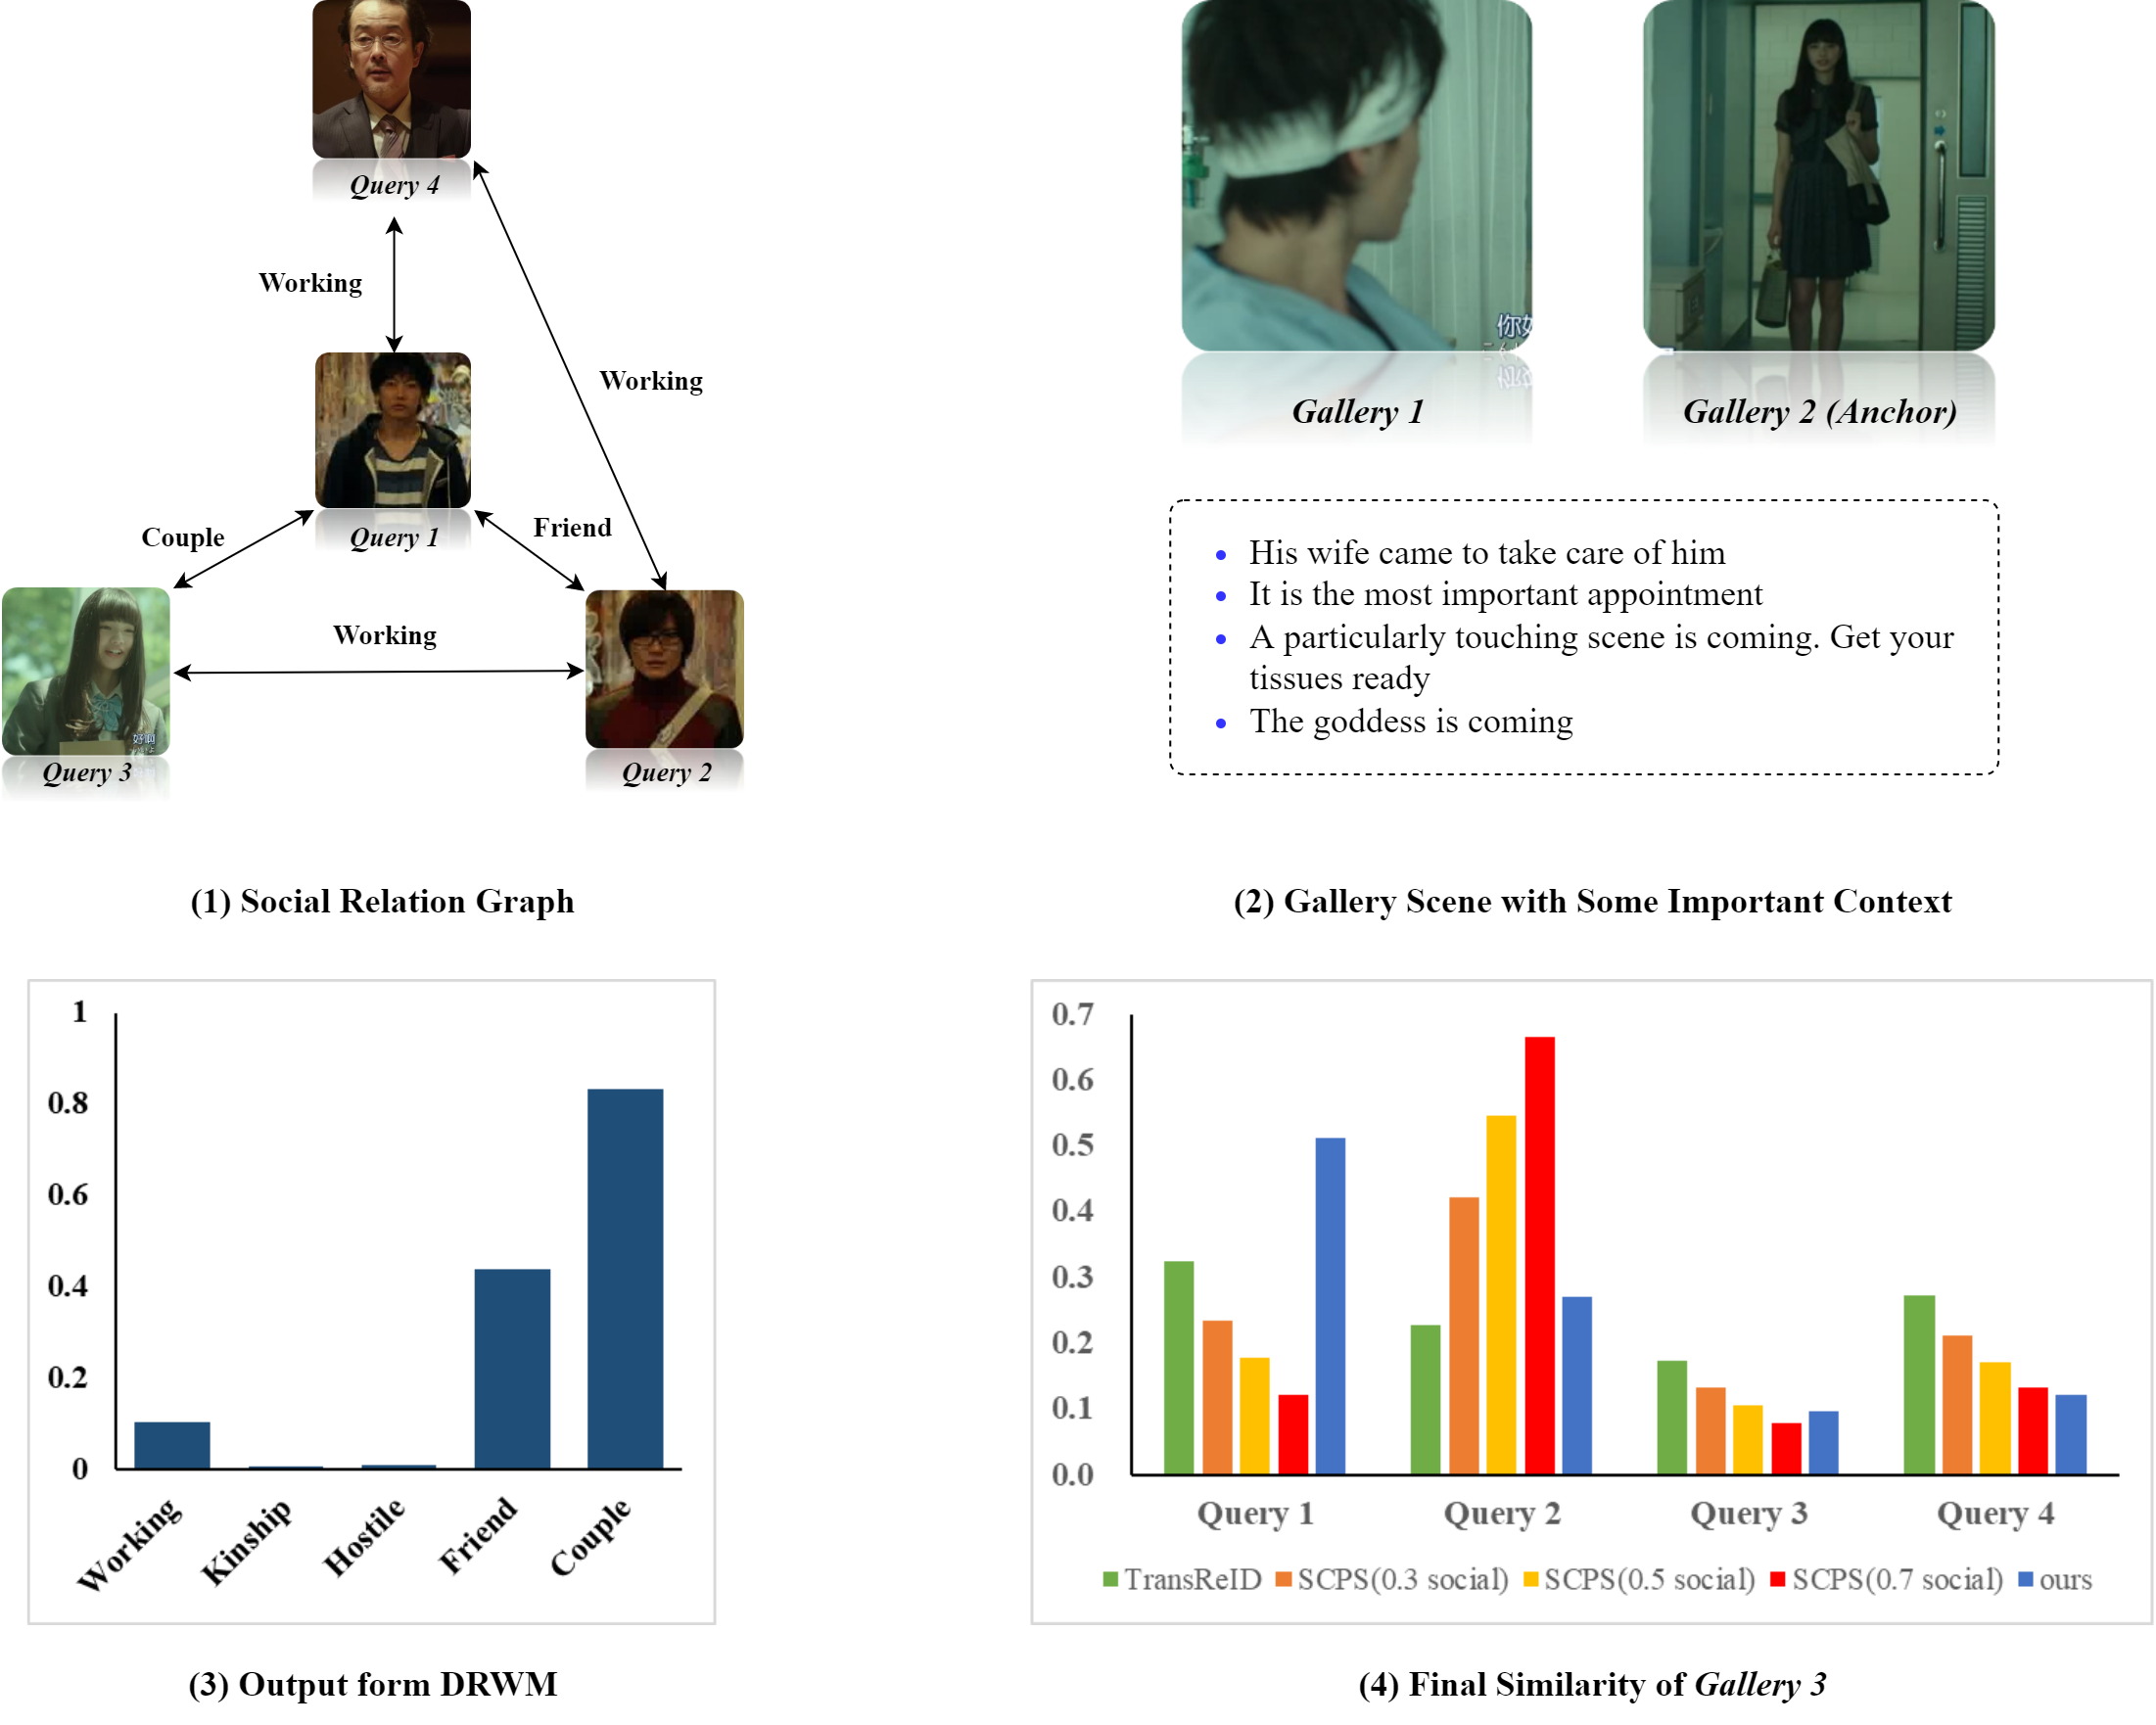}
	\caption{Case 1: Performance on movie "Bakuman". The green, orange, yellow, red and blue columns represent the results of TransReID, SCPS with 0.3 social weight, SCPS with 0.5 social weight, SCPS with 0.7 social weight and our method respectively}
	\label{case1}
\end{figure}
\begin{figure}[h]
	\centering
	\includegraphics[width=\linewidth]{./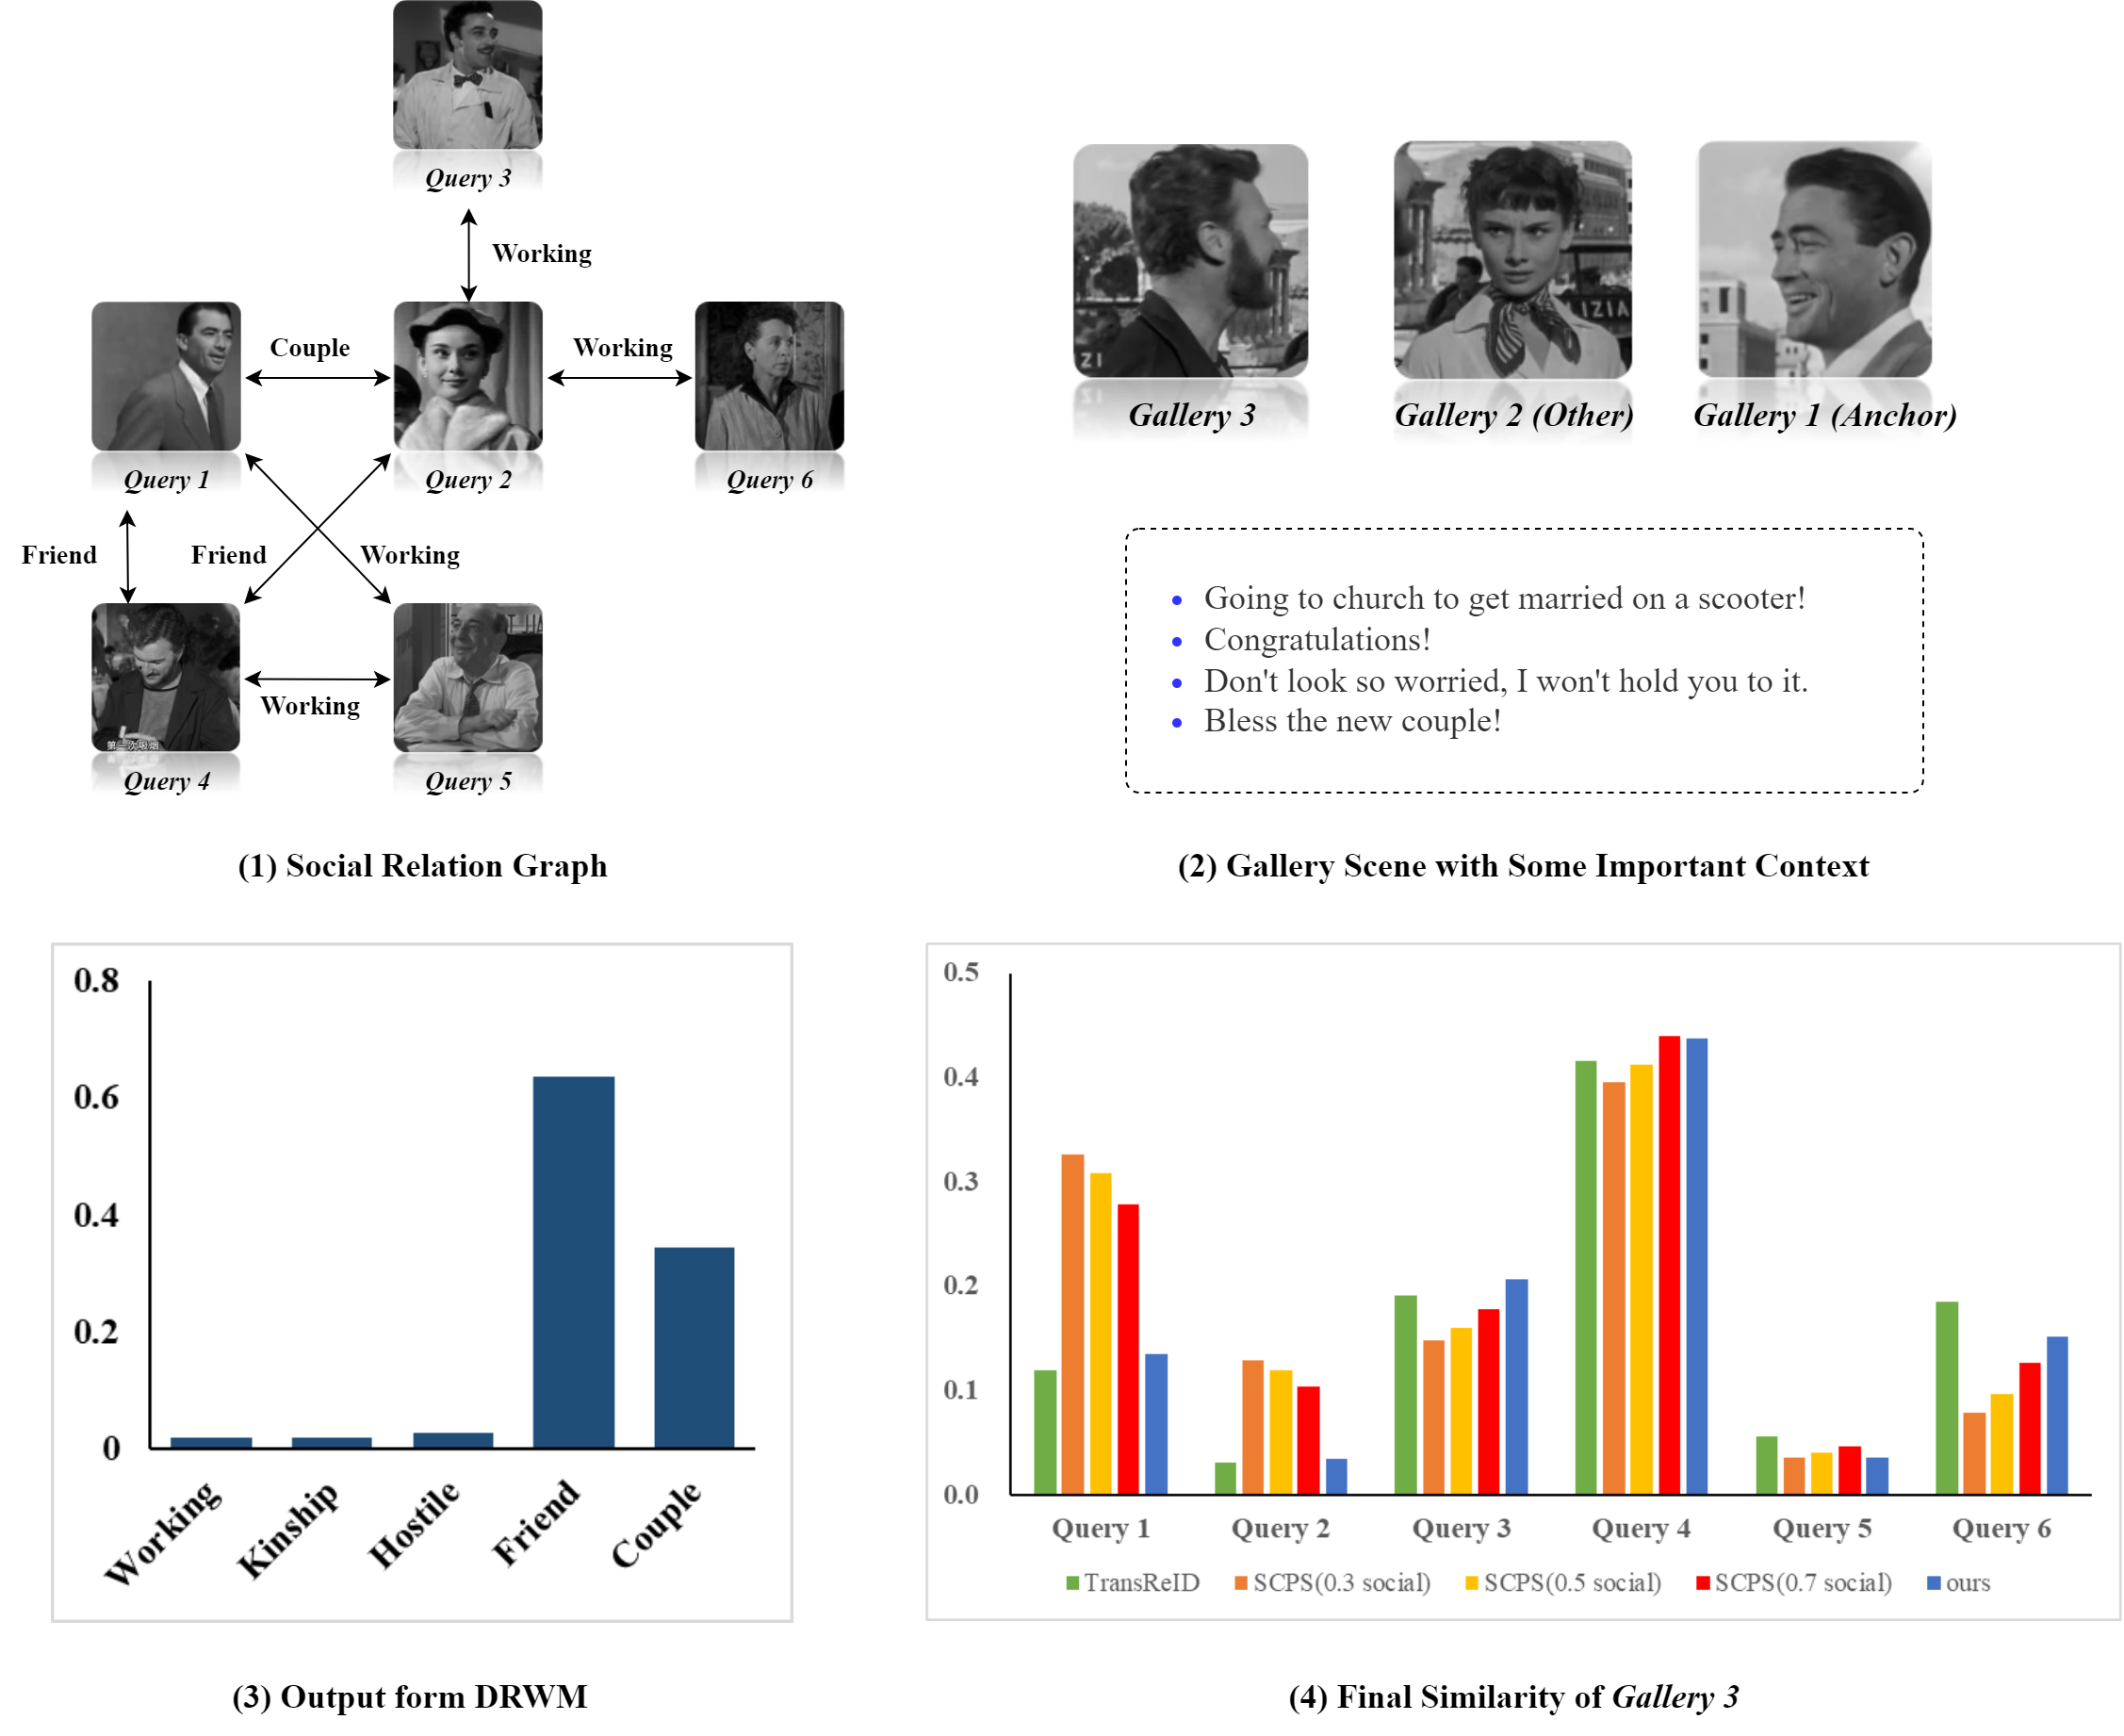}
	\caption{Case 2: Performance on movie "Roman Holiday".The green, orange, yellow, red and blue columns represent the results of TransReID, SCPS with 0.3 social weight, SCPS with 0.5 social weight, SCPS with 0.7 social weight and our method respectively}
	\label{case2}
\end{figure}
\subsection{Case Study}
In this section, we demonstrate two examples in detail to prove the effectiveness of our method. As shown in Figures \ref{case1} and \ref{case2}, we show four parts of each example, respectively: (1) The predefined social relationship graph; (2) The gallery characters in the scene and the context that can help us infer their identities or relationships; (3) The possibility of different relationships output from DRWM according to the context; (4) Similarity output from TransReID, SCPS with different social similarity weights and ours method. In addition, it is worth noting that the search task is a ranking task rather than a classification task. Therefore, models need to improve the similarity of the corresponding query-gallery pair as much as possible.\par
Figure \ref{case1} is a scene in the Japanese movie $"Bakuman"$. In this scene, $gallery_2 (query_3)$ comes to the hospital to visit the injured $gallery_1 (query_1)$. Since the camera focused on $gallery_2$ then, the visual model could easily identify her as query3. However, $gallery_1$ only shows his back. It is difficult to speculate its identity if only visual information is used, which is why TransReID performs poorly. As we can see, much information in the context implies the relationship between the two. Therefore, DRWM speculates that the most likely social relationship in this scene is $"couple"$. And we can narrow the search scope of gallery1 identity to the couple of $query_3$. Correspondingly, according to the social relation graph, we know that $query_1$ is the couple of $query_3$. Hence, our model improves the similarity of $query_1-gallery_1$. However, the SCPS needs to recognize the similarity of all query-gallery pairs and gallery-gallery pairs, and any misjudgment of a pair of relationships may lead to the failure of the label propagation. And it introduces excessive social similarity and wrongly improves the similarity of $query_2-gallery_1$.\par

Figure \ref{case2} is a scene in the American movie $"Roman Holiday"$. There are three characters in the scene, namely, $gallery_1 (query_1)$, $gallery_2 (query_2)$ and $gallery_3 (query_4)$. Among them, $gallery_1$ and $gallery_2$ are relatively easy to identify, while $gallery_3$ does not expose his face, which makes it difficult to obtain his identity directly. In this scene, COM selects gallery1 as the anchor to identify $gallery_3$. Furthermore, DRWM speculates that the most likely relationship is $"friend"$ and $"couple"$ through rich context. Therefore, we can narrow the search scope of $gallery_3$ to friend and couple of $query_1$. Correspondingly, in the predefined social relation graph, we find that $query_4$ and $query_2$ are friend and couple of $query_1$ respectively. Hence, compared with TransReID, SPCS and our method increase the similarity between $query_4-gallery_3$ and $query_1-gallery_3$. As mentioned, the SCPS cannot control the proportion of social similarity well and wrongly increased the similarity of $query_1-gallery_3$. However, since the social weight of our model is affected by the anchor identity probability and the probability of relationships, it does not cause the similarity of $query_1-gallery_3$ to increase excessively.
